# Supplementary material for: Generative News Recommendation
Source: arXiv:2403.03424 source file (2024-03-06)
Supplement: Supplementary file 1 [file appendix.tex]

\appendix
\section{Example prompts}
\begin{table*}[h]
\caption{Example prompts for multi-news narrative generation}\label{tab:fuse_prompt}
\small

\begin{tabular}{>{\centering\arraybackslash}p{15cm}}
\rowcolor{yellow!20}
\hline
\multicolumn{1}{c}{\textbf{Instruction}}                                                                                                                                                                                                                                                                                                                                                                                                                                                                                                                                                                                                                                                                                                                                                                                                                                                                                                                                                                                                                                                                                                                                                                                                     \\ \hline
\rowcolor{yellow!2}
\begin{tabular}[c]{@{}l@{}}You are a personalized text generator. First, I will provide you with a news list that includes both the \textbf{{[}main news{]}} and \\ \textbf{{[}topic-related news{]}}. Second, I will provide you with user interests, including the \textbf{{[}categories{]}} and \textbf{{[}topics{]}} of news that the user\\ is interested in. Based on the input news list and user interests, you are required to generate a \textbf{\{personalized news summary\}} \\ centered around the \textbf{{[}main news{]}}.\end{tabular}                                                                                                                                                                                                                                                                                                                                                                                                                                                                                                                                                                                                                                                                                                                                                           \\ \hline
\rowcolor{violet!10}
\multicolumn{1}{c}{\textbf{Input}}                                                                                                                                                                                                                                                                                                                                                                                                                                                                                                                                                                                                                                                                                                                                                                                                                                                                                                                                                                                                                                                                                                                                                                                                           \\ \hline

\begin{tabular}[c]{@{}l@{}}News List:\\ \{"ID": "Main News", "title": "Lionel Messi says he wants to continue ‘living a few more games being world champion’", \\ "abstract": "Ever since he was a young boy growing up in Rosario, Lionel Messi’s ultimate dream ...", "topic": "Messi ..."\}\\ \{"ID": "Topic-related News 1", "title": "How the world reacted to ‘the best World Cup final ever’", "abstract": "This World \\ Cup final was a game that seemed to defy comprehension, conventions and any attempt ...", "topic": "the World Cup final..."\}\\ \{"ID": "Topic-related News 2", "title": "Lionel Messi cements his place among the greats after winning epic duel against Kylian \\ Mbappé", "abstract": "Now there can be no arguments. Now there should be no debate. In the ...", "topics": "Lionel Messi ..."\}\\ \{"ID": "Topic-related News 3", "title": "Why Argentina’s win over France was the greatest World Cup final ever", "abstract": \\ "It seems only yesterday that Enner Valencia was swatting aside Qatar in the 2022 World Cup...", "topics": "World Cup ..."\}\\ User Interest:\\ This user is interested in news about{[}sports{]}, especially {[}Lionel Messi, Argentina national football team{]}.\end{tabular} \\ \hline
\rowcolor{violet!20}
\multicolumn{1}{c}{\textbf{Output}}                                                                                                                                                                                                                                                                                                                                                                                                                                                                                                                                                                                                                                                                                                                                                                                                                                                                                                                                                                                                                                                                                                                                                                                                          \\ \hline
\rowcolor{violet!2}
\begin{tabular}[c]{@{}l@{}}"title": "Lionel Messi Desires to Continue 'Living a Few More Games Being World Champion",\\ "category": "sports", "topic": "Lionel Messi, Argentina national football team, World Cup final",\\ "abstract": "\textbf{Lionel Messi}, who recently achieved his lifelong dream of winning the \textbf{World Cup for Argentina}, expressed his \\ desire to continue 'living a few more games being world champion.' This victory, marked by several brilliant individual \\ performances from \textbf{Messi}, has been celebrated globally. The final match, which included an intense duel with Kylian Mbappé,\\  is being hailed as one of the most memorable \textbf{World Cup finals}."\end{tabular}                                                                                                                                                                                                                                                                                                                                                                                                                                                                                                                                                              \\ \hline

\end{tabular}
\end{table*}
